# Supplementary material for: Diffusion Generative Models in Infinite Dimensions
Source: arXiv:2212.00886 source file (2023-02-24)
Supplement: Supplementary file 1 [file appendix.tex]

\section{Some Computational Lemmas}

The following lemma shows us that the forward process is tractable and has well-behaved distributions. This extends some of the computations of \citet{ho2020denoising} to the functional setting.
\begin{lemma} \label{lemma:basic_gp_computations}
Consider the process defined by Equation \eqref{eqn:forward_markov_chain}. Let $\gamma_t = \prod_{i=1}^t (1 - \beta_t)$ to simplify the notation. We have the following facts:
\begin{itemize}
    \item The conditional distribution of $u_{t} | u_{t-1}$ is $\mathcal{GP}(\sqrt{1 - \beta_t} u_{t-1}, \beta_t K)$.
    \item The conditional distribution of $u_t | u_0$ is $\mathcal{GP}(\sqrt{\gamma_t} u_0, (1 - \gamma_t) K)$.
\end{itemize}
\end{lemma}
\begin{proof}
The claimed relationships hold for finite-dimensional Gaussians. Since the vector space operations on $\mathcal{GP}$ act pointwise, they will hold for all finite index sets, and hence will hold for the overall $\mathcal{GP}$s.
\end{proof}

A slightly more difficult but important lemma: the true reverse-chain is tractable conditioned on data $u_0$. The finite-dimensional version of the following lemma is stated (without proof) in \citet{ho2020denoising}. In the finite-dimensional setting, there is a much simpler proof using Bayes' theorem and the resulting closed-form densities -- however, this proof does not work in the infinite-dimensional setting due to the lack of canonical reference measure in $\hilb$. I suspect there is a cleaner proof than what is presented below, but this is good enough. Note also that this lemma has the finite-dimensional case as a special case (we can just take the GP to have a finite index set).

\begin{lemma} \label{lemma:double_conditioned_backwards}
In the setting of the previous lemma, for $t \geq 2$,
\begin{equation}
    u_{t-1} | u_t, u_0 \sim \mathcal{GP}\left(\widetilde{\mu_t}(\blank | u_t, u_0), \widetilde{\beta_t}K \right)
\end{equation}
where the mean function is given by 
\begin{equation}
    \widetilde{\mu_t}(\blank | u_t, u_0) = \frac{\sqrt{\gamma_{t-1}}\beta_t }{1 - \gamma_t} u_0(\blank) + \frac{\sqrt{1 - \beta_t}(1 - \gamma_{t-1})}{1 - \gamma_t} u_t(\blank)
\end{equation}
and the covariance function is
\begin{equation}
    \widetilde{\beta_t}K = \frac{1 - \gamma_{t-1}}{1 - \gamma_t} \beta_t K.
\end{equation}

\end{lemma}
\begin{proof}

By Lemma \eqref{lemma:basic_gp_computations}, we know that
\begin{equation} \label{eqn:step1}
    u_{t-1} = \sqrt{\gamma_{t-1}}u_0 + \sqrt{1 - \gamma_{t-1}} \xi
\end{equation}
and by construction we have
\begin{equation} \label{eqn:step2}
    u_t = \sqrt{1 - \beta_t} u_{t-1} + \sqrt{\beta_t} \xi'
\end{equation}

where $\xi, \xi' \sim \mathcal{GP}(0, K)$ are independent draws. Our strategy is to manipulate these expressions to obtain a reparametrized expression for $u_{t-1}$. By Equation \eqref{eqn:step1},
\begin{equation} \label{eqn:step3}
    \beta_t \sqrt{\gamma_{t-1}} u_0 = \beta_t \left[u_{t-1} - \sqrt{1 - \gamma_{t-1}} \xi \right],
\end{equation}
and similarly by Equation \eqref{eqn:step2},
\begin{equation} \label{eqn:step4}
    (1 - \gamma_{t-1}) \sqrt{1 - \beta_t} u_t = (1 - \gamma_{t-1}) \left[ (1 - \beta_t) u_{t-1} + \sqrt{\beta_t} \sqrt{1 - \beta_t} \xi' \right].
\end{equation}

Upon summing Equations \eqref{eqn:step3}-\eqref{eqn:step4} and isolating the $u_{t-1}$ terms,
\begin{align}
    \left(\beta_t + (1 - \gamma_{t-1})(1 - \beta_t) \right) u_{t-1} &= \beta_t \sqrt{\gamma_{t-1}} u_0 + (1 - \gamma_{t-1}) \sqrt{1 - \beta_t} u_t \\
    &+ \beta_t \sqrt{1 - \gamma_{t-1}} \xi - (1 - \gamma_{t-1}) \sqrt{\beta_t}\sqrt{1 - \beta_t} \xi' \nonumber.
\end{align}

On the LHS, we have
\begin{align} \label{eqn:step5}
    (\beta_t + (1 - \gamma_{t-1})(1 - \beta_t)) u_{t-1} &= (\beta_t + (1 - \beta_t) - (1-\beta_t)(\gamma_{t-1}))u_{t-1} \nonumber \\
    &= (1 - \gamma_t) u_{t-1}
\end{align}

thereby allowing us to obtain
\begin{align}
    u_{t-1} &= \frac{\beta_t \sqrt{\gamma_{t-1}}}{1 - \gamma_t}u_0 + \frac{\sqrt{1 - \beta_t} (1 - \gamma_{t-1})}{1 - \gamma_t} \\
    &+ \frac{\beta_t \sqrt{1 - \gamma_{t-1}}}{1 - \gamma_t}\xi - \frac{(1 - \gamma_{t-1}) \sqrt{\beta_t}\sqrt{1 - \beta_t}}{1 - \gamma_t} \xi'.
\end{align}

We now analyize the noise terms (i.e. those depending on $\xi, \xi'$). It is clear that the noise terms have mean zero. Moreover, this is the sum of two scaled, independent standard $\mathcal{GP}$s, and hence it is a $\mathcal{GP}$ with covariance
\begin{align*}
    &\left(\frac{\beta_t \sqrt{1 - \gamma_{t-1}}}{1 - \gamma_t} \right)^2 + \left(\frac{(1 - \gamma_{t-1}) \sqrt{\beta_t} \sqrt{1 - \beta_t})}{1 - \gamma_t} \right)^2 \\
    &= \left(\frac{\beta_t(1 - \gamma_{t-1})}{1 - \gamma_t}\right)\left( \frac{\beta_t + (1-\beta_t)(1 - \gamma_{t-1})}{1 - \gamma_t}\right) \\
    &= \frac{\beta_t(1 - \gamma_{t-1})}{1 - \gamma_t}
\end{align*}

where the last line follows from the calculation in Equation \eqref{eqn:step5}.
\end{proof}

We also note that it is straightforward to reparameterize the mean as
\begin{equation} \label{eqn:reparam_mean}
    \widetilde{\mu_t}(\blank | u_t(u_0, \xi), u_0) = \widetilde{\mu_t}(\blank | u_t, \xi) = \frac{1}{\sqrt{1 - \beta_t}} \left(u_t(\blank | u_0, \xi) - \frac{\beta_t}{\sqrt{1 - \gamma_t}} \xi(\blank) \right)
\end{equation}

\section{Kernels and their Spectra}

To implement our methods it will be useful to have code that computes the eigenvalues and eigenfunctions of some common kernels. Note that the eigenvalues and eigenfunctions depend on the input space $(\XX, \mu)$, where $\mu$ is assumed to be a finite measure on $\XX$, i.e. such that $\mu(\XX) < \infty$. The main examples of interest (at least for now) are $\XX = \R$ with $\mu = \mathcal{N}(0, 1)$, and $\XX = [a, b]$ with $\mu = \d x$ being the Lebesgue measure. It would be great to obtain analytical expressions for the eigenvalues and eigenfunctions of the following kernels on those state spaces:
\begin{itemize}
    \item Squared-Exponential kernel (aka RBF):
    \begin{equation}
        k(x, x') = \sigma^2 \exp \left[ -\frac{1}{2} \frac{||x - x'||_2^2}{\ell^2}  \right] \qquad \sigma^2, \ell \in \R
    \end{equation}
    An expression is given for $(\XX, \mathcal{N}(0, 1))$ in \cite[Chapter~4.3.1]{williams2006gaussian}.
    \item Mat\'ern Kernel:
    \begin{equation}
        k(x, x') = \frac{\sigma^2}{2^{\nu - 1} \Gamma(\nu)} \left( \frac{\sqrt{2 \nu}}{\ell} ||x - x'||_2 \right)^\nu K_\nu \left(\frac{\sqrt{2 \nu}}{\ell} ||x - x'||_2 \right)
    \end{equation}
    See \cite[Chapter~4]{williams2006gaussian} for details on this expression.
\end{itemize}

It might also be interesting/useful to implement some kind of numerical method to estimate the eigentuples of arbitrary kernels, e.g. the Nystr\"om method, see \cite[Chapter~4.3.2]{williams2006gaussian}.


\subsection{Closed-Form Kernel Expressions}

\begin{enumerate}
    \item Let $\XX = \R$ with $\mu = \mathcal{N}(0, s^2)$. Take the squared-exponential kernel
    \begin{equation}
        k(x, x') = \sigma^2 \exp \left[ -\frac{1}{2} \frac{||x - x'||_2^2}{\ell^2}  \right] \qquad \sigma^2, \ell \in \RP.
    \end{equation}
    An expression for the eigenfunctions and eigenvalues is given in \cite[Chapter~4.3.1]{williams2006gaussian}.
    \item Let $\XX = [a, b]$ with $\mu = \UU[a, b]$ being the uniform measure. Take $k$ to be the Mat\'ern kernel with $\nu = 1/2$, i.e.
    \begin{equation}
        k(x, x') = \sigma^2 \exp \left( - \frac{||x - x'||_2}{\ell} \right) \qquad \sigma^2, \ell \in \RP.
    \end{equation}
    \citet[Section~2.1.3]{le2010spectral} gives closed-form expressions for the eigenvalues and eigenfunctions.
\end{enumerate}
